# Supplementary material for: Piko: A Design Framework for Programmable Graphics Pipelines
Source: arXiv:1404.6293 ancillary file (2015-01-30)
Supplement: Supplementary file 1 [file Piko-supplementary-material.pdf]

# Supplementary Materials: Synthesized Pipelines Using Piko

## 1 Introduction

In this document, we present source code for our forward-raster pipeline as described in the main paper and compiled using `Pikoc` as well as potential pipeline schedules for alternative graphic renders. The source code can be found in the compressed zip archive submitted along with this document.

For the potential pipeline schedules, each of the following sections discusses the general, architecture-independent features of each pipeline, as well as how the Piko pipeline definition changes for different implementation targets/objectives. While not all of these pipelines were implemented to the point of actual scene-rendering execution, we have defined each pipeline using the Piko definition, analyzed these definitions to produce the pipeline skeleton, and determined the kernel mapping using the Piko optimizer. We present the pipeline skeletons and kernel mappings for each pipeline in the sections below.

## 2 Triangle Rasterizer

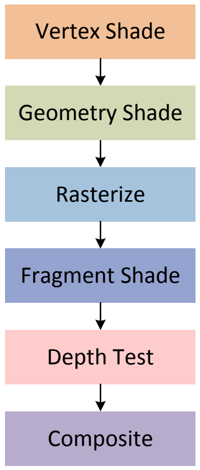


**Figure 1:** *This figure presents the high-level stage graph of a triangle rasterization pipeline.*

The first pipeline we present is a simple triangle rasterization pipeline. Figure 1 shows the graph of this pipeline. Using the same stage structure, we can define this pipeline in multiple ways such that each definition exploits different optimization opportunities.

## 2.1 Baseline

| Stage | Phase | Directive |
|---|---|---|
| Vertex Shade | `AssignBin` | Empty |
| Fullscreen bins | `Schedule` | `Load Balance`<br>`tileSplitSize` = 1024 |
| | `Process` | |
| Rasterize | `AssignBin` | `AssignPreviousBins` |
| Fullscreen bins | `Schedule` | `Load Balance`<br>`tileSplitSize` = 1024 |
| | `Process` | `processOneToMany` |
| Fragment Shade | `AssignBin` | `AssignPreviousBins` |
| Fullscreen bins | `Schedule` | `Load Balance` |
| | `Process` | |
| Depth Test | `AssignBin` | `AssignPreviousBins` |
| Fullscreen bins | `Schedule` | `Load Balance` |
| | `Process` | |
| Composite | `AssignBin` | `AssignPreviousBins` |
| Fullscreen bins | `Schedule` | `Load Balance`<br>`EndBin` |
| | `Process` | Custom |

**Table 1:** *The Piko directives for each stage in the* Baseline *version of the triangle rasterization pipeline.*

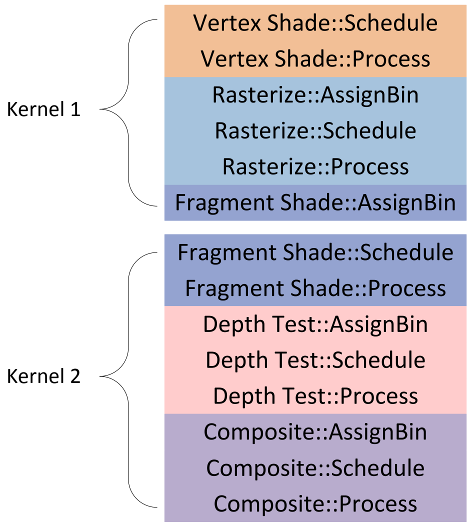


**Figure 2:** *The kernel mapping of the* Baseline *version of the triangle rasterization pipeline.*

The Baseline version of the triangle rasterization pipeline is very basic and does not make use of 2D tiling. Instead, the entire screen space is considered a single bin, and we launch batches of work in a load balanced fashion by splitting up the primitives. When implemented, this pipeline definition turns out to be similar FreePipe [Liu et al. 2010] (although Rasterize and Fragment Shade don't merge). The Piko directives for this pipeline are listed in Table 1.

We use this pipeline as a basis to demonstrate the options that Piko provides to customize pipeline execution based on different goals (such as preferring locality over load balance, or vice versa, as discussed below). Figure 2 shows the kernel mapping and execution order for the Baseline pipeline. Even though this pipeline does not utilize spatial binning, we can still exploit producer-consumer locality by fusing kernels.

## 2.2 Locality

| Stage | Phase | Directive |
|---|---|---|
| Vertex Shade | `AssignBin` | Empty |
| Fullscreen bins | `Schedule` | `Load Balance`<br>`tileSplitSize` = 1024 |
| | `Process` | |
| Geometry Shade | `AssignBin` | Custom |
| 128 × 128 bins | `Schedule` | `Load Balance` |
| | `Process` | Empty |
| Rasterize | `AssignBin` | Custom |
| 128 × 128 bins | `Schedule` | `Direct Map`<br>`scheduleBatch(32)` |
| | `Process` | |
| Fragment Shade | `AssignBin` | `AssignPreviousBins` |
| 128 × 128 bins | `Schedule` | `Direct Map`<br>`scheduleBatch(32)` |
| | `Process` | |
| Depth Test | `AssignBin` | `AssignPreviousBins` |
| 128 × 128 bins | `Schedule` | `Direct Map` |
| | `Process` | |
| Composite | `AssignBin` | `AssignPreviousBins` |
| 128 × 128 bins | `Schedule` | `Direct Map`<br>`EndBin` |
| | `Process` | Custom |

**Table 2:** *The Piko directives for each stage in the Locality version of the triangle rasterization pipeline.*

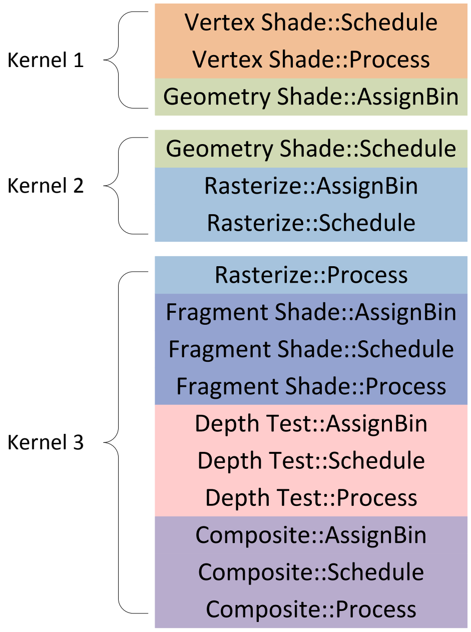


**Figure 3:** *The kernel mapping of the Locality version of the triangle rasterization pipeline*

We can also write the triangle rasterization pipeline in such a way as to prefer locality. Table 2 shows the directives that specify such a pipeline. The kernel mapping in Figure 3 shows that this pipeline prefers to fuse stages in order to preserve producer-consumer locality as much as

possible. Furthermore, because the screen is divided into bins, spatial locality provides further opportunity for performance increase through local fragment and depth buffers.

## 2.3 Load Balance

| Stage | Phase | Directive |
|---|---|---|
| Vertex Shade<br>Fullscreen bins | `AssignBin` | Empty |
| | `Schedule` | `LoadBalance`<br>`tileSplitSize` = 1024 |
| | `Process` | |
| Geometry Shade<br>128 × 128 bins | `AssignBin` | Custom |
| | `Schedule` | `LoadBalance` |
| | `Process` | Empty |
| Rasterize<br>128 × 128 bins | `AssignBin` | Custom |
| | `Schedule` | `DirectMap`<br>`scheduleBatch(32)` |
| | `Process` | |
| Fragment Shade<br>128 × 128 bins | `AssignBin` | `AssignPreviousBins` |
| | `Schedule` | `LoadBalance`<br>`scheduleBatch(32)` |
| | `Process` | |
| Depth Test<br>128 × 128 bins | `AssignBin` | `AssignPreviousBins` |
| | `Schedule` | `DirectMap` |
| | `Process` | |
| Composite<br>128 × 128 bins | `AssignBin` | `AssignPreviousBins` |
| | `Schedule` | `DirectMap`<br>`EndBin` |
| | `Process` | Custom |

**Table 3:** *The Piko directives for each stage in the Load Balance vesion of the triangle rasterization pipeline*

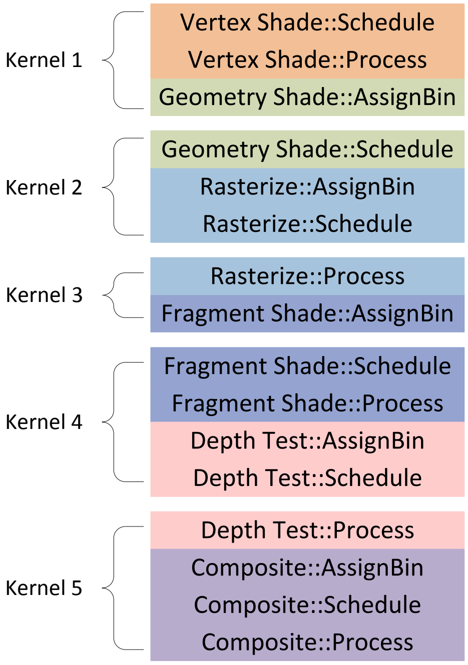


**Figure 4:** *The kernel mapping of the Load Balance version of the triangle rasterization pipeline.*

In the Load Balance triangle rasterization pipeline, we prefer to distribute the workload for Fragment Shader across the machine rather than keeping data localized to specific cores. While this version does not exploit locality as much as the Locality version, the Load Balance pipeline excels when the implementation target has a large number of cores. The directives in Table 3 lead to the kernel mapping in Figure 4, which shows reduced kernel fusion when compared to the Locality pipeline. However, by splitting stages into more kernels, this pipeline has more opportunity to redistribute workloads throughout execution.

# 3 Triangle Rasterizer with Deferred Shading

We now present multiple versions of a deferred rasterizer, a model that is popular for rendering complex effects in modern games [Lauritzen 2010]. Deferred shading is also utilized in the design of some modern mobile GPUs [Imagination Technologies Ltd. 2011]. We present three versions of Piko synthesis: a programmable multi-kernel implementation, a bucketing tiled-deferred renderer for mobile implementation, an OGL/D3D based implementation, and a programmable multi-kernel implementation.

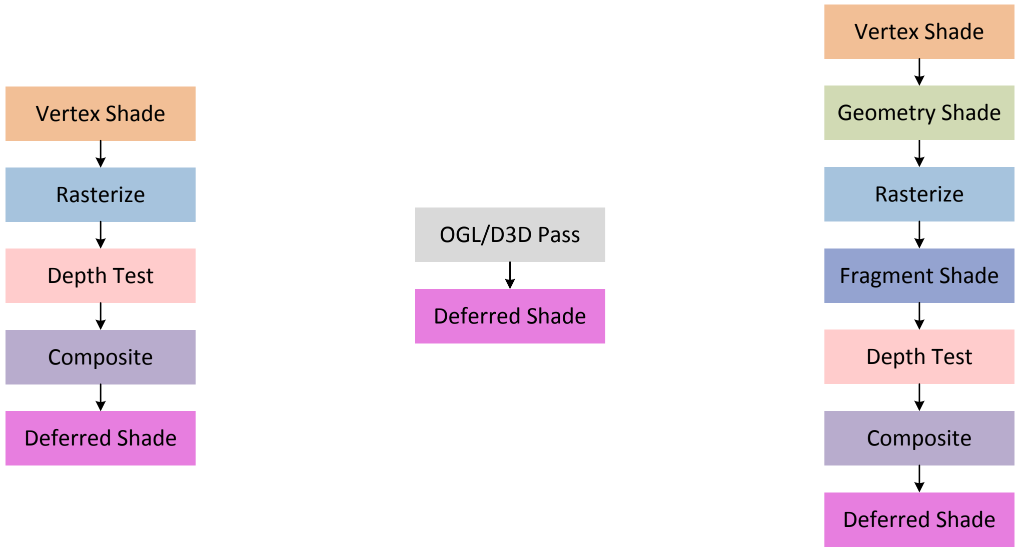


**Figure 5:** *These figures present the high-level stage graph for three types of deferred triangle rasterizers.*

## 3.1 Bucketing Deferred Renderer

Figure 5 left shows the higher level pipeline. Unlike a discrete version, there is no pre-visibility shading. Table 4 lists the Piko priorities of this pipeline, where the first stage uses `scheduleAll` to invoke depth-first bin processing. Figure 6 shows the final kernel organization.

| Stage | Phase | Directive |
|---|---|---|
| Vertex Shade $8 \times 8$ bins | `AssignBin` | Custom |
| | `Schedule` | `scheduleAll` `tileSplitSize` = 1024 |
| | `Process` | |
| Rasterize $8 \times 8$ bins | `AssignBin` | Custom |
| | `Schedule` | `DirectMap` `scheduleBatch(32)` |
| | `Process` | `processOneToMany` |
| Depth Test $8 \times 8$ bins | `AssignBin` | `assibnPreviousBins` |
| | `Schedule` | `DirectMap` |
| | `Process` | |
| Composite $8 \times 8$ bins | `AssignBin` | `assibnPreviousBins` |
| | `Schedule` | `DirectMap` `EndBin` |
| | `Process` | |
| Deferred Shade $8 \times 8$ bins | `AssignBin` | `assibnPreviousBins` |
| | `Schedule` | `DirectMap` `EndBin` |
| | `Process` | Custom |

**Table 4:** *The Piko directives for each stage in the Bucket version of the deferred triangle rasterizer pipeline.*

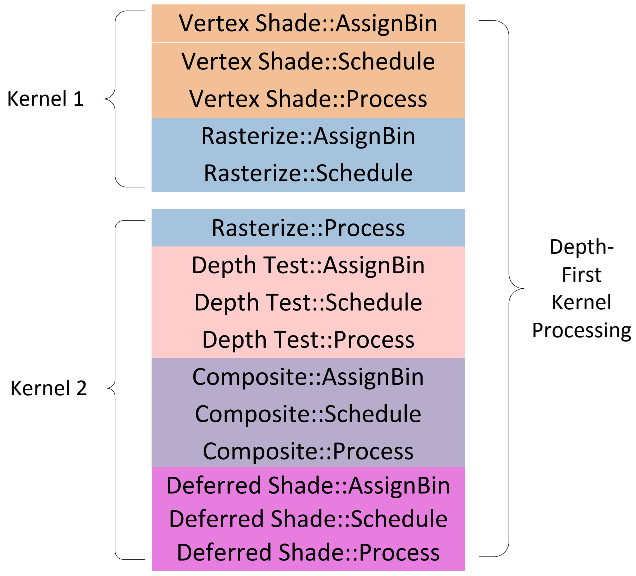


**Figure 6:** *The kernel mapping of the Bucket version of the deferred triangle rasterizer pipeline.*

### 3.2 OGL/D3D-based Implementation

| Stage | Phase | Directive |
|---|---|---|
| OGL/D3D Pass<br>Fullscreen bins | AssignBin | Empty |
| | Schedule | Serialize |
| | Process | Custom |
| Deferred Shade<br>$8 \times 8$ bins | AssignBin | Custom |
| | Schedule | LoadBalance<br>EndBin |
| | Process | Custom |

**Table 5:** *The Piko directives for each stage in the OGL/D3D version of the deferred triangle rasterizer pipeline.*

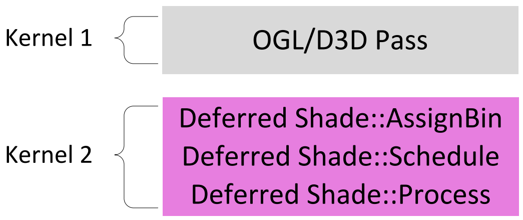


**Figure 7:** *The kernel mapping of the OGL/D3D-based deferred raster.*

An OGL/D3D (Figure 5 middle)pipeline uses the fixed-function GPU pipeline for an initial pass, and shades the results in an added stage. Table 5 shows the Piko preferences for such a pipe, and Figure 7 shows the final kernel mapping.

### 3.3 Load-balanced Multi-Kernel Implementation

Our final implementation builds on our rast-locality model by adding a Deferred Shade stage at the end of the pipeline. Figure 5 right shows the structure of this pipeline, and Table 6 shows the Piko directives. Figure 8 shows the synthesized output. Note that Deferred Shader fuses with Composite despite the EndBin dependence.

| Stage | Phase | Directive |
|---|---|---|
| Vertex Shade<br>Fullscreen bins | AssignBin | Empty |
| | Schedule | schedulescheduleAll<br>tileSplitSize = 1024 |
| | Process | |
| Geometry Shade<br>$128 \times 128$ bins | AssignBin | Custom |
| | Schedule | scheduleLoadBalance |
| | Process | Empty |
| Rasterize<br>$8 \times 8$ bins | AssignBin | Custom |
| | Schedule | scheduleDirectMap<br>scheduleBatch(32) |
| | Process | processOneToMany |
| Fragment Shade<br>$8 \times 8$ bins | AssignBin | assibnPreviousBins |
| | Schedule | scheduleLoadBalance<br>scheduleBatch(32) |
| | Process | |
| Depth Test<br>$8 \times 8$ bins | AssignBin | assibnPreviousBins |
| | Schedule | scheduleDirectMap |
| | Process | |
| Composite<br>$8 \times 8$ bins | AssignBin | assibnPreviousBins |
| | Schedule | scheduleDirectMap<br>EndBin |
| | Process | |
| Deferred Shade<br>$8 \times 8$ bins | AssignBin | assibnPreviousBins |
| | Schedule | scheduleDirectMap<br>EndBin |
| | Process | Custom |

**Table 6:** *The Piko directives for each stage in the Load Balance version of the deferred triangle rasterizer pipeline.*

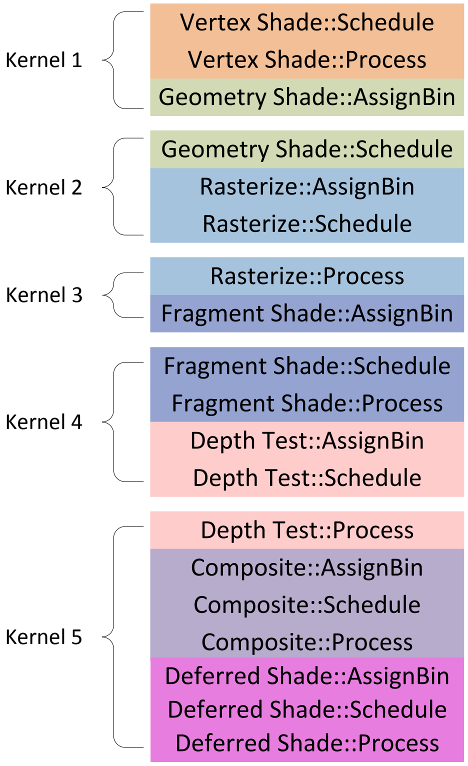


**Figure 8:** *The kernel mapping of the Load Balance version of the deferred triangle rasterizer pipeline.*

# 4 Reyes Renderer

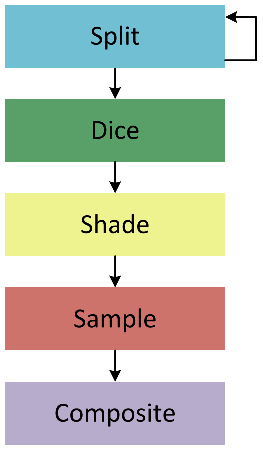


**Figure 9:** *This figure represents the high-level stage graph of a Reyes pipeline.*

The Reyes pipeline [Cook et al. 1987] provides an example pipeline that differs in structure from the previous two. The Split stage of this pipeline cycles back to itself as many times as necessary to appropriately prepare data for the Dice stage. This cycle presents another kernel mapping challenge, because it prevents fusion and will iterate a variable number of times. In addition, the number of primitives that result from the Split stage can grow to a large value such that standard breadth-first processing is either impossible (due to memory constraints) or high inefficient (due to lost locality). To resolve these issues, we may employ depth-first bin processing, which not only speeds up execution by improving locality, but also allows this pipeline to run on hardware with limited memory.

## 4.1 Many-core Reyes Renderer

| Stage | Phase | Directive |
|---|---|---|
| Split<br>Fullscreen bins | `AssignBin` | Empty |
| | `Schedule` | `scheduleLoadBalance`<br>`tileSplitSize = 8` |
| | `Process` | `processOneToMany` |
| Dice<br>Fullscreen bins | `AssignBin` | `assibnPreviousBins` |
| | `Schedule` | `scheduleLoadBalance`<br>`tileSplitSize = 8` |
| | `Process` | |
| Shade<br>Fullscreen bins | `AssignBin` | `assibnPreviousBins` |
| | `Schedule` | `scheduleLoadBalance`<br>`tileSplitSize = 8` |
| | `Process` | |
| Sample<br>128 × 128 bins | `AssignBin` | `assibnPreviousBins` |
| | `Schedule` | `scheduleLoadBalance`<br>`tileSplitSize = 8` |
| | `Process` | `processOneToMany` |
| Composite<br>128 × 128 bins | `AssignBin` | `assibnPreviousBins` |
| | `Schedule` | `DirectMap`<br>`tileSplitSize = 8`<br>`scheduleEndBin` |
| | `Process` | Custom |

**Table 7:** *The Piko directives for each stage in the Many-core Reyes Renderer.*

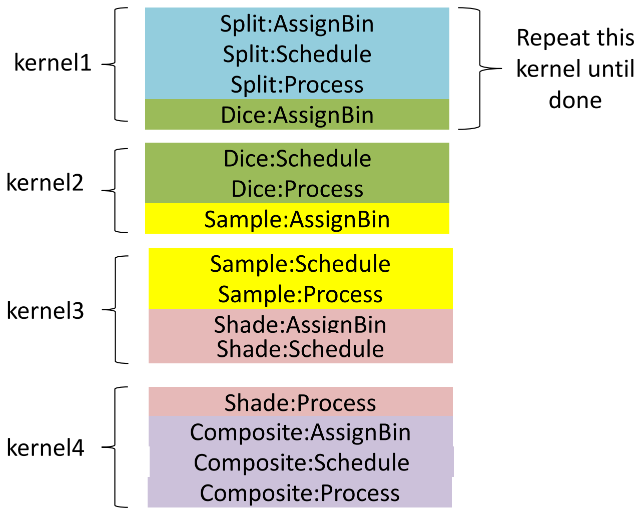


**Figure 10:** *The kernel mapping of the Many-core Reyes Renderer.*

Dice's `AssignBin` phase is placed in the same kernel as Split. When patches are deemed ready to be diced, then the Split phase will run Dice's `AssignBin` and place the patches in bins.

## 4.2 Bucket Reyes Renderer

| Stage | Phase | Directive |
|---|---|---|
| Split<br>128 × 128 bins | `AssignBin` | Custom |
| | `Schedule` | `All`<br>`tileSplitSize` = 256 |
| | `Process` | |
| Dice<br>128 × 128 bins | `AssignBin` | `AssignPreviousBins` |
| | `Schedule` | `All`<br>`tileSplitSize` = 256 |
| | `Process` | |
| Shade<br>128 × 128 bins | `AssignBin` | `AssignPreviousBins` |
| | `Schedule` | `All`<br>`tileSplitSize` = 256 |
| | `Process` | |
| Sample<br>32 × 32 bins | `AssignBin` | `AssignPreviousBins` |
| | `Schedule` | `All`<br>`tileSplitSize` = 256 |
| | `Process` | |
| Composite<br>32 × 32 bins | `AssignBin` | `AssignPreviousBins` |
| | `Schedule` | `All`<br>`EndBin` |
| | `Process` | Custom |

**Table 8:** *The Piko directives for each stage in the bucket Reyes renderer.*

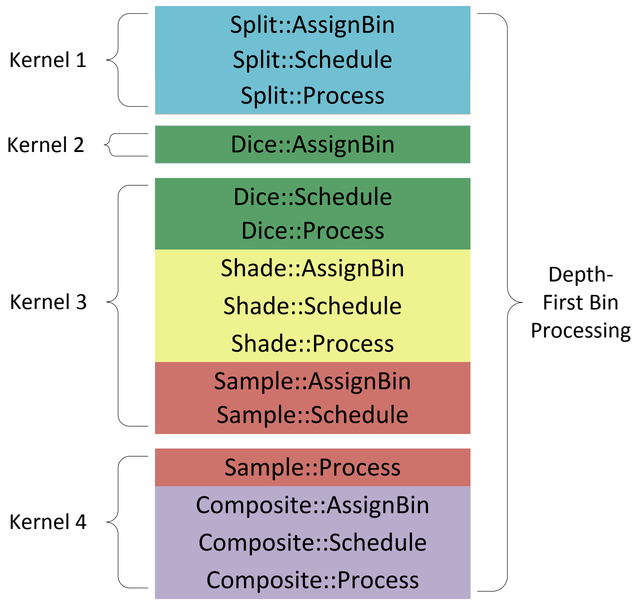


**Figure 11:** *The kernel mapping of the bucket Reyes renderer.*

This version of the pipeline can also run on many-core environments and is similar to RenderAnts [2009], but it is geared towards scenes with high complexity. Thus, the pipeline uses buckets to restrict its working set. This strategy both preserves producer-consumer locality and reduces memory requirements by preferring to push data as far through the pipeline as possible before selecting another bucket. The directives needed to specify a bucketing Reyes renderer are shown in Table 8.

In contrast to the kernel mapping for the many-core Reyes renderer (Figure 10), the bucket Reyes pipeline kernel mapping (Figure 11) chooses to fuse kernels to preserve producer-consumer locality. Also, the mapping indicates that bins should be processed depth-first, again to preserve locality.

# 5 Ray Tracing

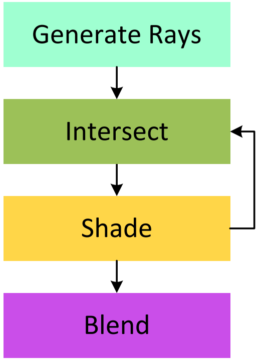


**Figure 12:** *This figure presents the high-level stage graph of a ray trace pipeline.*

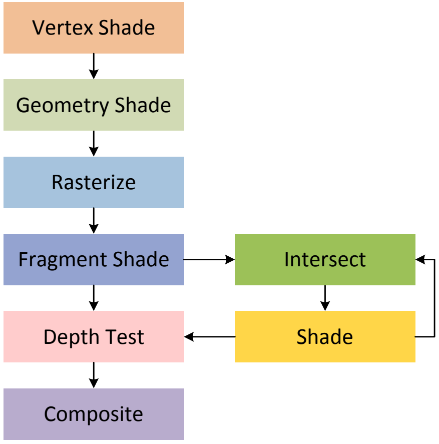


**Figure 13:** *This figure presents the high-level stage graph of a hybrid rasterization/ray trace pipeline.*

We now present kernel mappings for a simple ray tracer, and hybrid pipeline that extends a forward rasterizer with a ray tracer for secondary rays. The latter design is based on the extension proposed by authors of GRAMPS [Sugerman et al. 2009].

## 5.1 Simple Ray Tracer

| Stage | Phase | Directive |
|---|---|---|
| GenRays Fullscreen bins | `AssignBin` | Empty |
| | `Schedule` | `LoadBalance` `tileSplitSize` = 4096 |
| | `Process` | Custom |
| Intersect $16 \times 16$ | `AssignBin` | `AssignPreviousBins` |
| | `Schedule` | `LoadBalance` |
| | `Process` | |
| Shade $16 \times 16$ | `AssignBin` | `AssignPreviousBins` |
| | `Schedule` | `LoadBalance` |
| | `Process` | |
| Blend $16 \times 16$ | `AssignBin` | `AssignPreviousBins` |
| | `Schedule` | `DirectMap` |
| | `Process` | Custom |

**Table 9:** *The Piko directives for each stage in the Ray Tracer.*

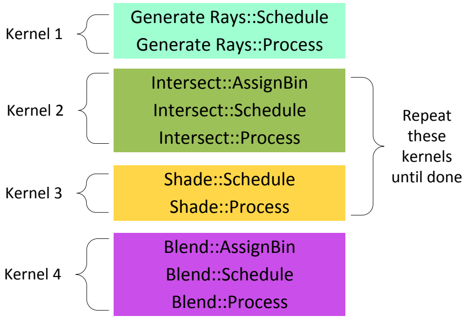


**Figure 14:** *The kernel mapping of the ray trace pipeline*

Figure 12 shows the higher level pipeline, and Table 9 shows the Piko mappings for the pipeline. The resulting kernel mapping is shown in Figure 14. Note the loop that allows processing of secondary, tertiary, etc. rays.

### 5.2 A Hybrid Rasterizer-Ray Tracer

| Stage | Phase | Directive |
|---|---|---|
| Vertex Shade<br>Fullscreen bins | AssignBin | Empty |
| | Schedule | Load Balance<br>tileSplitSize = 1024 |
| | Process | |
| Geometry Shade<br>128 × 128 bins | AssignBin | Custom |
| | Schedule | Load Balance |
| | Process | Empty |
| Rasterize<br>128 × 128 bins | AssignBin | Custom |
| | Schedule | Direct Map<br>scheduleBatch(32) |
| | Process | |
| Fragment Shade<br>128 × 128 bins | AssignBin | AssignPreviousBins |
| | Schedule | Load Balance<br>scheduleBatch(32) |
| | Process | |
| Intersect<br>16 × 16 | AssignBin | AssignPreviousBins |
| | Schedule | Load Balance |
| | Process | |
| rtshade<br>16 × 16 | AssignBin | AssignPreviousBins |
| | Schedule | Load Balance |
| | Process | processOneToMany |
| Blend<br>16 × 16 | AssignBin | AssignPreviousBins |
| | Schedule | Direct Map |
| | Process | Custom |
| Depth Test<br>128 × 128 bins | AssignBin | AssignPreviousBins |
| | Schedule | Direct Map |
| | Process | |
| Composite<br>128 × 128 bins | AssignBin | AssignPreviousBins |
| | Schedule | Direct Map<br>EndBin |
| | Process | Custom |

**Table 10:** *The Piko directives for each stage in a hybrid Rasterizer and Ray Tracer pipeline.*

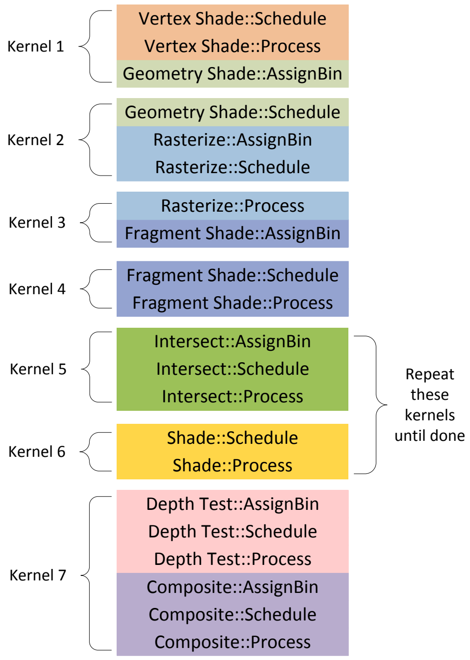


**Figure 15:** *The kernel mapping of the hybrid rasterization/ray trace pipeline*

We synthesize a simple rasterizer with extensions for ray tracing from the Fragment Shader (Figure 13). In a scene, some surfaces may use regular forward shading techniques, while others may use a ray tracer. The Depth Test and Composite stages merge the outputs from the two paths. Table 10 lists the scheduling policies for these stages, and Figure 15 shows the final kernel mapping.

## References


COOK, R. L., CARPENTER, L., AND CATMULL, E. 1987. The Reyes image rendering architecture. In *Computer Graphics (Proceedings of SIGGRAPH 87)*, 95–102.

IMAGINATION TECHNOLOGIES LTD. 2011. *POWERVR Series5 Graphics SGX architecture guide for developers*, 5 July. Version 1.0.8.

LAURITZEN, A., 2010. Deferred rendering for current and future rendering pipelines. [Beyond Programmable Shading, SIGGRAPH 2010].

LIU, F., HUANG, M.-C., LIU, X.-H., AND WU, E.-H. 2010. FreePipe: a programmable parallel rendering architecture for efficient multi-fragment effects. In *I3D '10: Proceedings of the 2010 ACM SIGGRAPH Symposium on Interactive 3D Graphics and Games*, 75–82.

SUGERMAN, J., FATAHALIAN, K., BOULOS, S., AKELEY, K., AND HANRAHAN, P. 2009. GRAMPS: A programming model for graphics pipelines. *ACM Transactions on Graphics 28*, 1 (Jan.), 4:1–4:11.

ZHOU, K., HOU, Q., REN, Z., GONG, M., SUN, X., AND GUO, B. 2009. RenderAnts: Interactive Reyes rendering on GPUs. *ACM Transactions on Graphics 28*, 5 (Dec.), 155:1–155:11.
